# Supplementary material for: Large electropositive cations as surfactants for the growth of polar epitaxial films
Source: arXiv:1412.3422 source file (2014-12-10)
Supplement: Supplementary file 1 [file Supplemental.pdf]

# Supplemental Material:

Large electropositive cations as surfactants for the growth of polar epitaxial films

Alfred K. C. Cheung, Ilya Elfimov, Mona Berciu, and George A. Sawatzky

## 1 Potassium coverage beyond 1/2 per unit cell

For completeness, we consider what happens if more potassium is adsorbed than the minimum of 1/2 per unit cell needed for compensation of the polar problem. In Figs. 1 and 2, we plot the Ti and K projected densities of states (PDOS) near $E_F$ at three values of K coverage: 1/2 per unit cell (the case discussed in the Letter), as well as 3/4 and 1 per unit cell, respectively. The thickness of the LAO layer is $m = 2$.

For the latter two cases, Fig. 1 shows that although the K overlayer now has sufficient electrons to transfer more than 1/2 electron per unit cell to the interface, the conduction electron density at the interface is found to be essentially the same as in the former case. Correspondingly, electron density is retained in the K overlayer for the higher coverages beyond 1/2 K per unit cell, as expected (Fig. 2). This agrees with the picture of K donating just enough electrons to compensate for the diverging potential. Anything beyond that would result in energetically expensive overcompensation.

The energetic favorability for further K adsorption can be quantified by calculating the additional cohesive energy upon adsorption of extra K atoms. In particular, we take as a reference 4 unit cells of LAO/STO with 2 adsorbed K atoms (1/2 K per unit cell coverage), whose total energy we denote by $E_{K_2[LAO_2STO_4]_4}$. We can now further adsorb 1 or 2 more K atoms onto this system to attain 3/4 and 1 per unit cell K coverage. We denote the total energies of these systems by $E_{K_3[LAO_2STO_4]_4}$ and $E_{K_4[LAO_2STO_4]_4}$, respectively. The extra cohesive energies upon adsorption of each additional K can then be defined as:

$$E_{coh,3/4} = E_{K_3[LAO_2STO_4]_4} - E_{K_2[LAO_2STO_4]_4} - E_K \tag{1}$$

$$E_{coh,4/4} = E_{K_4[LAO_2STO_4]_4} - E_{K_3[LAO_2STO_4]_4} - E_K, \tag{2}$$

where $E_K$ is the energy of an isolated K atom.

We find that $|E_{coh,3/4}| = 1.36$ eV and $|E_{coh,4/4}| = 1.53$ eV. These are to be contrasted with the cohesive energy per adsorbed K for the first two adsorbed K atoms, which was calculated to be 2.2 eV (see Fig. 4 of Letter). The cohesive energy as defined is approximately 0.7-0.8 eV smaller for K atoms adsorbed beyond the critical 1/2 per unit cell coverage, i.e. it is much less energetically favorable for extra K atoms to be adsorbed onto the system. As mentioned in the conclusion of the Letter, this observation is critical for preventing any undesired accumulation of K onto the surface. In particular, the large cohesive energy difference between K atoms adsorbed up to 1/2 coverage and

K atoms adsorbed beyond 1/2 coverage suggests that if the substrate temperature is kept higher than some critical threshold, then any extra K will evaporate off. This would prevent a thick layer of K metal from forming on the surface and hence fundamentally changing the system.

## 2 Projected densities of states at different LAO thicknesses

In Fig. 3 of the Letter, we plotted the *total* DOS for the system, both with and without K, for LAO thicknesses $m = 1, 2, 3, 4, 5$, and 6. In Fig. 3 below we show the corresponding projected DOS onto Ti, O, and surface K (for the case with K adsorption). As expected, we find that the conduction band is of mostly Ti (3d) character. The main message of Fig. 3 in the Letter is retained: in the case without K adsorption, the Ti 3d conduction band moves to lower energy as the LAO thickness increases. It eventually crosses the Fermi energy (referenced at 0) to form the interface conducting electron gas at a critical thickness near $m = 4$. In contrast, the case with K stays mostly the same for all LAO thicknesses as a result of K donating its 4s electron and compensating for the polar problem starting from one unit layer of LAO.

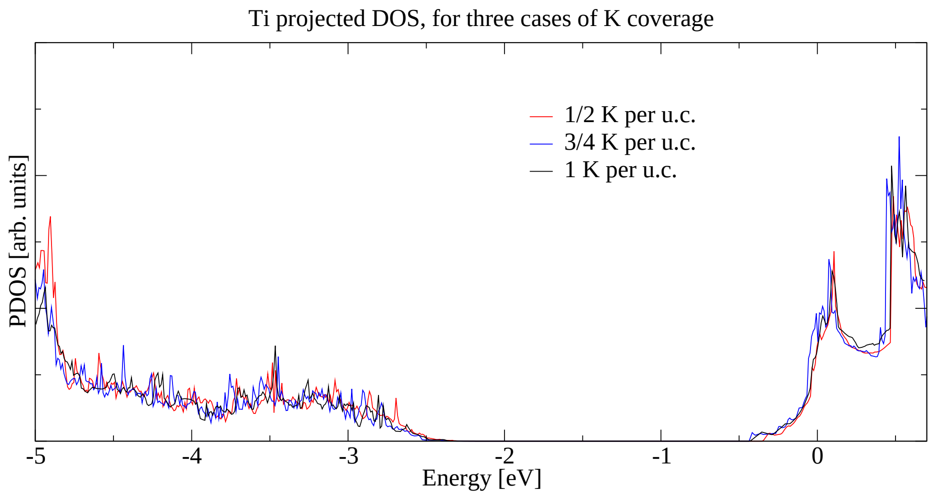


Figure 1: Ti PDOS near the Fermi energy, at three cases of K coverage, for LAO thickness of two unit layers. The density of conduction electrons in Ti remains the same for all three cases. This indicates that K adsorption beyond the critical amount needed for the ideal exact compensation does not result in extra electrons being transferred to the interface. Electron donation beyond what is needed would be overcompensation.

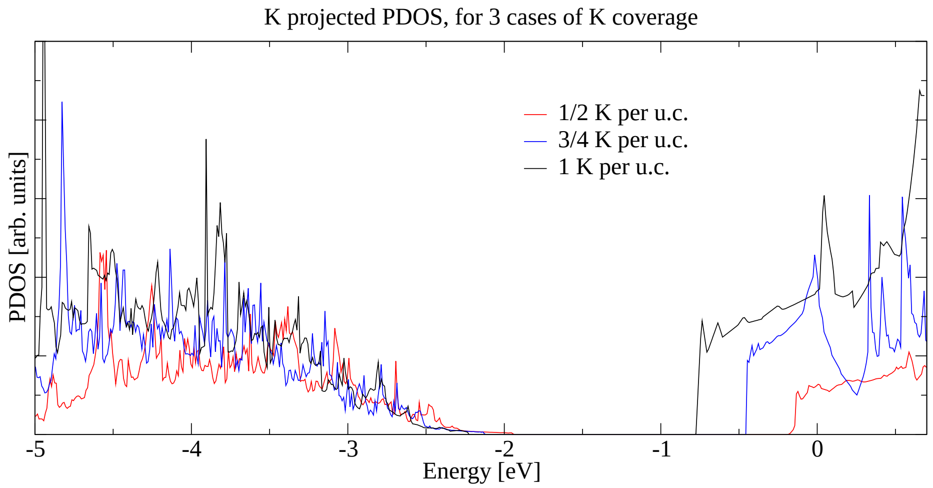


Figure 2: K PDOS near the Fermi energy, at three cases of K coverage, for LAO thickness of two unit layers. The density of conduction electrons retained by K increases significantly going from 1/2 to 3/4 per unit cell coverage, and then from 3/4 to 1 per unit cell coverage. This is in accordance with Fig. 1: K adsorption beyond the critical amount needed for the ideal exact compensation does not result in extra electrons being transferred to the interface; the extra electrons remain in the K overlayer.

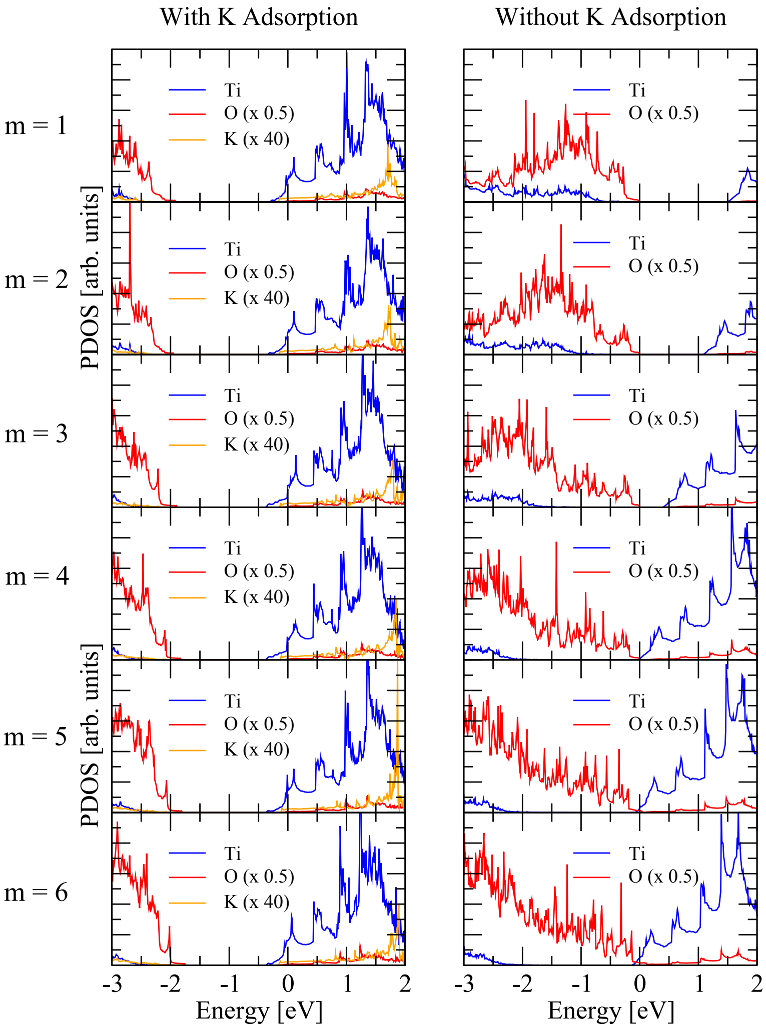


Figure 3: Ti, O, and surface K PDOS for the system, both with and without K, for LAO thicknesses $m = 1, 2, 3, 4, 5$, and 6. The Fermi energy is at 0. As pointed out in the Letter, although the plot may seem to depict a significant conduction electron density remaining at the surface K overlayer, note that the K PDOS is scaled up by a factor of 40. Thus, the residual electron density at K is greatly exaggerated.
